# Supplementary material for: Discommensuration-enhanced superconductivity in the charge density wave phases of transition-metal dichalcogenides
Source: arXiv:1806.08064 source file (2019-03-19)
Supplement: Supplementary file 1 [file G-L-theory-si.pdf]

# SUPPLEMENTARY MATERIAL

## Discommensuration-driven superconductivity in the charge density wave phases of transition-metal dichalcogenides

Chuan Chen,[1,2] Lei Su,[3] A. H. Castro Neto,[1,2] and Vitor M. Pereira[1,2]

[1] *Centre for Advanced 2D Materials and Graphene Research Centre, National University of Singapore, Singapore 117546*

[2] *Department of Physics, National University of Singapore, Singapore 117542*

[3] *Department of Physics, University of Chicago, Chicago, Illinois 60637, USA*

## CONTENTS

S1. General applicability of the approach to TMDs 3

S2. Transformation of the order parameter under symmetries of the system 5

S3. Free energy derived from the symmetries of the system 6

S4. The commensurate and incommensurate wavevectors in $TiSe_2$ 6

S5. Choice of the CDW free-energy parameters 7

S6. Mapping the lock-in energy to doping 10

S7. Harmonic expansion 11

S7.A. Outline of the method 11

S7.B. Explicit form of the harmonic-expanded free energy 13

S8. Solving for the equilibrium CDW order parameter 14

S9. Explicit form of the SC free energies 16

S10. On the coupling between superconductivity and CDW fluctuations 17

S11. Choice of the superconducting free energy parameters 18

S12. Solving for the equilibrium superconducting order parameter 19

S13. Real-space superconducting order 20

References 22

## S1. GENERAL APPLICABILITY OF THE APPROACH TO TMDS

It is important to highlight that the proposal discussed here to phenomenologically couple CDW and superconducting (SC) order is not specific or limited to $TiSe_2$. This means, for example, that our framework and qualitative outcome in terms of the correlation between superconductivity and the NC regime does not hinge in any way on a specific choice of $\mathbf{Q}_j^I$ and $\mathbf{Q}_j^C$, including their relative orientation.

In particular, note that the qualitatively most important contribution in this work is the concept that CDW fluctuations in the NC regime are either the driving mechanism of the superconducting pairing or, at least, are a significant factor in enhancing any underlying pairing (in the sense of BCS via electron-phonon). This is materialized in the proposed SC free energy ($\mathcal{F}_{\text{sc}}$, Eq. 3 of the main text), where the SC order parameter is directly coupled to the fluctuations of the CDW order which, in this Ginzburg-Landau approach, are manifest as DCs. Our presentation of this and the associated parameterization of $\mathcal{F}_{\text{sc}}$ make clear that there is nothing specific to $TiSe_2$. On the other hand, in order to have a specific connection with experiments and to demonstrate the power and completeness of this approach to describe qualitatively accurate phase diagrams, we have to make a specific choice. Such a choice turns out to be unavoidable in order to extract a phase diagram for the CDW order because the form of the interaction terms in the CDW free energy (Eqs. 2a and 2b) depends explicitly on the type of (in)commensurability condition. In our opinion, the best representative system is indeed $TiSe_2$, for the reasons stated in the main text: relatively high CDW and SC transition temperatures, reduced semi-metallic carrier densities that allow one to map the whole CDW and SC phase diagram as a function of doping, and its gate tunability in thin-film samples that allows full mapping of the temperature-density phase diagram using the same sample. This makes $TiSe_2$ arguably the currently best candidate to investigate the nature of the CDW/SC interplay, and also to validate or constrain our theory.

Notwithstanding, the fact that one must specify a particular (in)commensurability in order to generate a phase diagram does not detract from the general applicability of the approach described here because:

1. For example, if one intends to apply it to the case of 2H-$TaSe_2$, one needs only to re-write $f_2(\mathbf{r})$ in Eq. (2b) in the form appropriate to describe a $3 \times 3$ CDW, which has in fact been done by a number of authors in the past (for the CDW only)[1–3].

2. The fact that the CDW transition between the commensurate and incommensurate phases

takes place via an intermediate NC regime, as explicitly obtained here, is a universal aspect of this transition, irrespective of the commensurability conditions[3,4]. Therefore, the existence of localized DCs in the NC regime is a universal feature, and so are its implications for the nucleation of the SC order.

3. The above two points associate the appearance of superconductivity in experiments on closely related TMDs with the loss of commensurability of the background charge density wave. Our coupling scheme generates this outcome naturally because the superconducting order parameter is favoured in principle in near-commensurate and IC-CDW regimes where $\nabla \psi_j \neq 0$. This is actually verified by the behavior of other representative layered transition metal dichalcogenides, which are effectively two-dimensional from the electronic point of view. Consider, for example, the well known cases of $NbSe_2$ and $TaSe_2$,[5] or $TaS_2$[6]:

   (a) Under normal conditions (ambient pressure, undoped) 2H-$NbSe_2$ undergoes a transition to an IC CDW phase at $T_{\rm icdw} = 33$ K, which is followed by the onset of superconductivity at $T_{\rm sc} = 7.2$ K. No commensurate CDW phase is known to exist. The superconducting order appears and coexists within the ICDW state[7].

   (b) 2H-$TaSe_2$, on the other hand, has an ICDW transition at $T_{\rm icdw} = 120$ K, followed by a second transition to a commensurate CDW at $T_{\rm ccdw} = 90$ K[8]. However, this system has not been found to superconduct at any temperature which, within our scheme, is attributed to the fact the underlying CDW is commensurate.

   (c) 1T-$TaS_2$ has no superconductivity at ambient pressure and displays a commensurate CDW down to zero temperature. Under pressure, the commensurability is suppressed and superconductivity emerges in the near-commensurate regime. The phase diagram is qualitatively similar to that of $TiSe_2$ (see Fig. 3 of reference 6).

   These examples indicate a systematic *anti*-correlation between CDW commensurability and superconductivity, as can be also appreciated in Fig. 1 of reference 9, that compares the experimental $T_{\rm cdw}$ with $T_{\rm sc}$ for a representative set of these compounds.

These observations agree with the qualitative phase diagram predicted in our paper, namely: (i) SC is not stabilized in the CCDW state because it would need to energetically compete with it; (ii) systems that remain in the near-commensurate or IC-CDW state down to low temperatures eventually develop superconductivity. For example, unlike $TiSe_2$ and $TaS_2$ that have low carrier

density, $NbSe_2$ is an intrinsically good metal with high carrier density, and hence difficult to dope. Our model explains its experimental behavior upon lowering the temperature in a natural way: $NbSe_2$ is representative of a system with small lock-in energy sitting towards the right-hand side of our diagram and, consequently, goes first from the normal to an ICDW state, and afterwards becomes superconductor at low temperatures.

## S2. TRANSFORMATION OF THE ORDER PARAMETER UNDER SYMMETRIES OF THE SYSTEM

In order to establish a Ginzburg-Landau free energy, we begin with considering the symmetries of the system. Monolayer $TiSe_2$ has four types of symmetry: translational, $C_3$ rotation, mirror (along $\Gamma M$'s) and inversion. Using the fact that the commensurate wavevectors are $\mathbf{Q}_j^C \equiv \mathbf{G}_j/2$, where $\mathbf{G}_j$ $(j=1,2,3)$ are primitive reciprocal vectors related by 120 degree rotations, the order parameters transform as follows.

1. Under translation by a Bravais lattice vector,

$$\begin{aligned}\delta\rho'(\mathbf{r}) =& \delta\rho(\mathbf{r}-\mathbf{R}_{b.l})\\ =& \sum_j e^{i\frac{\mathbf{G}_j}{2}\cdot(\mathbf{r}-\mathbf{R}_{b.l})}\psi_j(\mathbf{r}-\mathbf{R}_{b.l}) + c.c\\ =& \sum_j e^{i\frac{\mathbf{G}_j}{2}\cdot \boldsymbol{r}} e^{-i\frac{\mathbf{G}_j}{2}\cdot\mathbf{R}_{b.l}}\psi_j(\mathbf{r}-\mathbf{R}_{b.l}) + c.c\\ \psi_j'(\mathbf{r}) =& e^{-i\frac{\mathbf{G}_j}{2}\cdot\mathbf{R}_{b.l}}\psi_j(\mathbf{r}-\mathbf{R}_{b.l})\end{aligned} \tag{S1}$$

2. Under a $C_3$ rotation,

$$\begin{aligned}\delta\rho'(\mathbf{r}) =& \delta\rho\left(C_3^{-1}\mathbf{r}\right)\\ =& \sum_j e^{i\frac{\mathbf{G}_j}{2}\cdot\left(C_3^{-1}\mathbf{r}\right)}\psi_j\left(C_3^{-1}\mathbf{r}\right) + c.c\\ =& \sum_j e^{i\frac{\mathbf{G}_{j-1}}{2}\cdot\mathbf{r}}\psi_j\left(C_3^{-1}\mathbf{r}\right) + c.c\\ =& \sum_j e^{i\frac{\mathbf{G}_j}{2}\cdot r}\psi_{j+1}\left(C_3^{-1}\boldsymbol{r}\right) + c.c\\ \psi_j'(\mathbf{r}) =& \psi_{j+1}\left(C_3^{-1}\mathbf{r}\right)\end{aligned} \tag{S2}$$

3. Under a mirror operation,

$$\begin{aligned}\psi_1'(x,y) =&\psi_1(-x,y)\\ \psi_2'(x,y) =&\psi_3(-x,y)\\ \psi_3'(x,y) =&\psi_2(-x,y)\end{aligned} \tag{S3}$$

4. Under an inversion, $\mathcal{I}$,

$$\psi_j'(\mathbf{r}) = \psi_j^*(-\mathbf{r}) \tag{S4}$$

## S3. FREE ENERGY DERIVED FROM THE SYMMETRIES OF THE SYSTEM

After taking into account the symmetry of the system in the spirit of references 3 and 10, assuming that higher order terms do not play a significant role, and only focusing on the simplest types of coupling which can capture the *lock-in* effect of the commensurate charge density wave (described by the $E$-term) and the interaction between the three density waves, one arrives at the free energy in Eq. (2):

$$\begin{aligned}f(x) =&A\sum_j|\psi_j|^2 + B\sum_j|\left(i\frac{\partial}{\partial x_{\parallel,j}} + \mathbf{q}_j^I\right)\psi_j|^2 + C\sum_j|\frac{\partial}{\partial x_{\perp,j}}\psi_j|^2 - \frac{3D}{2}\left(\psi_1\psi_2\psi_3 + \psi_1^*\psi_2^*\psi_3^*\right)\\ &- \frac{E}{2}\sum_j\left(\psi_j^2 + \psi_j^{*2}\right) + G\sum_j|\psi_j|^4 + \frac{K}{2}\sum_{i\neq j}|\psi_i\psi_j|^2 - \frac{M}{2}\sum_j\left(\psi_j\psi_{j+1}^*\psi_{j+2}^* + c.c\right)\end{aligned} \tag{S5}$$

In view of the $C_6$ rotational symmetry of the CDW and given that we are not interested in the development of other CDW phases due to induced anisotropy, strain, or disorder, we make the gradient term isotropic by choosing $B = C$.

## S4. THE COMMENSURATE AND INCOMMENSURATE WAVEVECTORS IN $TiSe_2$

As far as inelastic scattering is concerned, X-ray experiments in Cu-doped bulk samples by Joe *et al.*[11] and Kogar *et al.*[12], indicate that, while the incommensurability in the out-of-plane (stacking) direction is detectable experimentally beyond the critical doping, in-plane incommensurabilities were estimated to have too small a coherence length to be observable. Thus, inelastic scattering experiments in doped bulk crystals can only resolve an in-plane charge modulation with the commensurate $\mathbf{Q}^C$.

It should be stressed, however, that in a system that remains in the near-commensurate (NC) regime, the wavevector $\mathbf{Q}^I$ is only an abstract parameter in the theory, because the system never displays a uniform CDW with this wavevector. Instead, it remains locally commensurate with domain walls. As far as we can tell among all experiments in doped $TiSe_2$, this system is indeed either in the strictly commensurate or NC regime depending on the electronic density (these are limited to a maximum doping of less than 0.1 electrons per formula unit, either by the solubility limit in intercalated bulk samples, or by the gate capacitance in back-gate-tuned few-layer samples). Consequently, it is not surprising that bulk probes do not see CDW order with in-plane wavevector $\mathbf{Q}^I$, but only $\mathbf{Q}^C$, including in the NC regime. But, as we point out in our introduction, local probes (STM) do see DCs in the CDW phase at optimum SC doping, at temperatures above the SC dome, which favors the view that the system is in the NC-CDW regime when superconductivity emerges.

Transport signatures in ion-gel gated two-dimensional $TiSe_2$ indirectly suggest the presence of such domain-walls[13]. Subsequent STM experiments have directly shown the presence of intra-layer CDW DCs on surfaces of Cu-doped $TiSe_2$[14,15]. In the latter case, the DCs lines are perpendicular to the commensurate wavevector $\mathbf{Q}^C$, which implies that $\mathbf{Q}^I \parallel \mathbf{Q}^C$ is the correct choice in the model.

## S5. CHOICE OF THE CDW FREE-ENERGY PARAMETERS

Unlike a conventional Ginzburg-Landau theory for isotropic superconductors that requires only the specification of two independent phenomenological parameters (namely the gap and coherence length), the minimal free energy in Eqs. (2) necessary to reproduce the C / NC / IC-CDW transitions depends on a large number of parameters. This follows from the underlying physics because, even though we are not breaking the system's underlying $C_3$ rotational symmetry, the presence of three non-colinear density waves and their interactions dictates that one should consider all the terms in Eqs. (2). Therefore, an analysis of the full parameter space, in addition to being a formidable and unwieldy task, would only obfuscate the essential physics.

In addition to temperature ($T$), the experimental probes of the phase diagram are either doping ($x$) or pressure, but only the first is applicable to probing the intra-layer CDW order and superconductivity that we are considering here. We thus concentrate on the temperature − doping experimental phase diagrams, and analyze the predictions of our model in terms of variations of these two experimental parameters.

Temperature enters, as usual in a Ginzburg-Landau approach, linearly in the coefficient $A$ of $|\psi_j(\mathbf{r})|^2$,

$$A \equiv t \propto T - T_{\rm icdw}. \tag{S6}$$

By setting $A = t$ we are defining the energy units of the CDW free energy in terms of the reduced temperature, $t$, which has a direct relation to the experimental temperatures. As we explain in the main text, the largest influence of electron doping is expected to be in the lock-in energy which is controlled by the term proportional to the parameter $E$ in Eq. (2b). Hence, $E$ and $t$ become the parameters of interest in the theory to map into the experimental $x$ and $T$, respectively.

The above still leaves the parameters $B$, $G$, $D$, $M$ and $K$ unspecified in the CDW free energy, which require further consideration to determine the appropriate "slice" ($t$, $E$) to focus on for comparison with experiments within the whole multidimensional parameter space. In the absence, at the moment, of finer microscopic details from experiments regarding the near-commensurate regime and the large-scale distribution of discommensurations in $TiSe_2$, our main consideration is to avoid biasing the final solution towards a particular configuration. We therefore treat all terms in $\mathcal{F}_{\rm cdw}$ on equal footing by proceeding as follows.

1. Since we are mapping experimental changes in temperature and density to $A \equiv t$ and $E$, and since the various experimental phases are not fragile but consistently reproduced across different samples, as well as bulk and monolayers, these two parameters play the physically more dominant role in the phase diagram. For this reason, and given that the CDW transition occurs at $t \sim 0$, we explore the phase diagram in the region where $E$ is of the order of 1.

2. The parameter $B$ in Eq. (2a) sets the energy cost in deviating the charge modulation from the reference ICDW. In our approach to minimize the CDW free energy, the order parameter $\psi_j(\mathbf{r})$ is expanded in an harmonic series containing a variational wavevector $\mathbf{q}_j$ and all the harmonics thereof induced by the nonlinear terms in the free energy of Eq. (2) (see the details in supplementary section S7 below). Furthermore, recalling that: (i) $\mathbf{Q}_j^C \parallel \mathbf{G}_j$, (ii) that we are experimentally motivated to set $\mathbf{Q}_j^I \parallel \mathbf{Q}_j^C$ (see supplementary section S4) as well as to put $|\mathbf{Q}_1^I| = |\mathbf{Q}_2^I| = |\mathbf{Q}_3^I|$ to narrow the already large variational parameter space (also detailed in supplementary section S7), (iii) and recalling also the definition $\mathbf{q}_j^I \equiv \mathbf{Q}_j^I - \mathbf{Q}_j^C$, we have that $|\mathbf{q}_{1,2,3}^I| = q^I$, which is constant. Therefore, the second term in the free energy density $f_0(\mathbf{r})$ can be re-cast with the magnitude of $\mathbf{q}_j^I$ factored out as follows:

$$B\,(q^I)^2 \sum_j \left| \Big( \frac{i\,\boldsymbol{\nabla}_j}{q^I} + \frac{\mathbf{G}_j}{|\mathbf{G}_j|} \Big) \psi_j(\mathbf{r}) \right|^2, \tag{S7}$$

where the summand is now dimensionless. By setting the overall factor $B(q^I)^2 = 1$, we make this contribution to the free energy of the same order as the other terms.

3. We choose $M = -D$ to balance the two different types of phase relation between non-colinear waves. To see this, assume for a moment that all three density waves have the same amplitude, $\psi_j = \varphi e^{i\theta_j}$. The two terms in the free energy proportional to $M$ and $D$ become then:

$$-\frac{3D}{2}\cos(\theta_1+\theta_2+\theta_3) - \frac{M}{2}\left[\cos(\theta_1-\theta_2-\theta_3)+\cos(\theta_2-\theta_3-\theta_1)+\cos(\theta_3-\theta_1-\theta_2)\right],$$

   The lock-in ($E$) term favors $\theta_i$'s locked to multiples of $\pi$, i.e., $\theta_1 = m\pi, \theta_2 = n\pi, \theta_3 = l\pi$ with $m, n, l \in \mathbb{Z}$. By choosing $M = -D$, the $D$-term favors $m+n+l = 2k+1$ ($k \in \mathbb{Z}$), while the $M$-term favors $m+n+l = 2p$ ($p \in \mathbb{Z}$). Since they have similar order of magnitude, both types of phase configuration can appear in real space.

   This illustrates that the role of the free energy terms governed by the parameters $M$ and $D$ is to define how the three non-collinear waves interlock their phases in real space or, equivalently, the DCs along each of the three directions. Our choice leads to the Kagome pattern highlighted with the dashed lines in Fig. 2(a). Different choices, such as having $M$ and $D$ with the same sign and/or different magnitudes, translate into different periodic patterns of the DC network in real space. The important thing is that this affects only the precise arrangement of the DC network, and not the fact that there is a DC network. This means that changing the relative sign of $M$ and $D$ or their relative magnitudes (within reasonable bounds, see below) does not change the qualitative nature of the phase diagram. And, most importantly, it does not compromise the nucleation of the superconducting phase to the DCs that we describe in the main text (here too, different choices of these parameters lead only to different spatial profiles of the non-uniform SC order parameter, but not its suppression).

4. Numerical experimentation showed that the sequence of C-NC-IC transitions can be generated as shown in Fig. 1 by setting the magnitude of $B(q^I)^2$, $G$, $D$, $M$ and $K$ to 1, without qualitative changes in the features of the diagram (the phases stabilized, the sequence and order of transitions, overall topology of the phase diagram) within a comfortable range of variation in the magnitude of the parameters. We therefore settled on the final choice stated in the main text:

$$A = t, \quad K = G = 2M = -2D = 2, \quad B(q^I)^2 = 1. \tag{S8}$$

Note that all the parameters in the CDW free energy are thus of the same order of magnitude, with no particular one significantly larger or smaller than the others. In other words, there is no fine-tuning of parameters in order to capture a qualitatively correct phase diagram. This can be regarded as a result of building the free energy on well grounded physical considerations. Moreover, having all parameters of the order $\sim 1$ indicates that: (i) the phases and features shown in Fig. 1 are robust, (ii) the phase diagram shown Fig. 1 is not constrained *a priori* in any way to fit the experimental one.

Finally, and for completeness, we note that the magnitude of our parameters ($\sim 1$) is similar to that found by Nakanishi and Shiba in their earlier work that pioneered the systematic use of the harmonic expansion for the CDW order parameter in the context of 1T and 2H transition metal dichalcogenides[1,16]. As described in Supplementary Section "Harmonic Expansion", our treatment of the CDW order parameter consists of an implementation of their method, with the adaptation of including explicitly the harmonic component $\Delta_{j;0}$ to capture the C-CDW in the same expansion. Their work already establishes, across different materials, that the interesting transitions among the C, NC, and IC phases can be analyzed with all parameters $\sim 1$.

## S6. MAPPING THE LOCK-IN ENERGY TO DOPING

In the section "*CDW phase diagram*" of the main text we state the following: "*Physically, a* smaller $E$ *can be mapped to* larger *electron densities because: (i) phenomenologically, electron doping reduces the stability of the C state in favor of an IC-CDW*[12,13,15]*; (ii) the lock-in gain reflects the condensation energy of the C-CDW phase in a microscopic description, and the latter has been shown to decrease with doping in the excitonic theory for the C-CDW in* $TiSe_2$[17–20]". Below we elaborate on each of these statements in more detail.

"*(i) phenomenologically, electron doping reduces the stability of the C state in favor of an IC-CDW*" — This is a purely phenomenological consideration independent of any additional knowledge of the microscopic interactions that stabilize the commensurate CDW phase. It simply states that, in our model, $E$ is the parameter that, when reduced, weakens the stability of the commensurate phase in favor of a NC or incommensurate situation; experimentally, doping weakens the commensurate CDW; therefore, it is natural and reasonable to associate a decreasing $E$ with increased electronic density, on purely phenomenological grounds.

"*(ii) the phenomenological lock-in gain reflects the condensation energy of the C-CDW phase in a microscopic description, and the latter has been shown to decrease with doping in the excitonic*

*theory for the C-CDW in TiSe₂*" — In a microscopic description of the C-CDW transition (irrespective of whether it is driven by electron-phonon or electron-electron interactions), the gain in electronic energy (the so-called condensation energy at $T = 0$) is determined by the magnitude of the gap introduced in the bandstructure by the commensurate modulation of electronic density. In the microscopic formulation, the gap is the order parameter. On the other hand, in a Ginzburg-Landau model such as ours, the condensation energy is determined by $E$. This relationship between the lock-in parameter in the phenomenological treatment and the microscopic condensation energy is essentially the same in the CDW problem as in the Ginzburg-Landau approach to superconductivity. For the CDW case, it is discussed in detail, for example, in G. Grünner's textbook cited in the main text (see, in particular, section 7.1; see also references 17–19).

The essential point here is that there is a solid microscopic relationship between these two quantities, irrespective of the details of the model or target system. Now, in addition, in $TiSe_2$ the CDW gap decreases with doping. If this was simply a statement based on the experimental phase diagram, it would not be an independent argument. However, we also know from the specific microscopic calculations reported in reference 21 that the CDW gap/order parameter indeed decreases with doping. Therefore, there is a direct microscopic justification to map the decrease in $E$ with an increase in electron density, entirely at the theoretical level, independently of the experimental observations.

## S7. HARMONIC EXPANSION

### S7.A. Outline of the method

When we consider an IC-CDW characterized by a certain $\mathbf{q}_j$, the various terms in Eq. (2b) induce higher harmonics of it. Hence, the equilibrium IC state must consist of a linear combination of infinite compatible harmonics. This fact must be explicitly accounted for in order to properly describe: the C-IC transition, the fact that the equilibrium $\mathbf{q}_j$ changes with temperature, as well as the order of the phase transitions[5,22]. In addition, despite the insight provided by phase-only models[4,23], both the phase and amplitude of the order parameter should be considered to properly describe the stable CDW as, not a uniform plane wave solution, but a wave periodically distorted in real space to accommodate the competing $E$ and $B$ terms in the free energy[3,22,24]. These two aspects, combined with the fact that the saddle-point equations are nonlinear, make the analytical minimization of $f_{\text{cdw}}(\mathbf{r})$ a formidable problem, except in simplified cases[3,24].

A pragmatic approach consists in making a systematic harmonic expansion of the order parameter and minimizing the free energy numerically, as pioneered by Nakanishi *et al.*[1,16,25]. Accordingly, we consider the expansion

$$\psi_j\left(\boldsymbol{r}\right) = \Delta_{j;0} + \sum_{\substack{0\leq l,m,n\leq N\\ l\cdot m\cdot n=0}} \Delta_{j;lmn} \exp\!\big(i\mathbf{q}_{j;lmn}\cdot\mathbf{r}\big), \tag{S9}$$

where $\mathbf{q}_{j;lmn} \equiv (2l+1)\mathbf{q}_j + 2m\mathbf{q}_{j+1} + 2n\mathbf{q}_{j+2}$ are the harmonics of $\mathbf{q}_j$ generated by $f_1(\mathbf{r})$ and $l, m, n$ are positive integers smaller than a cutoff $N$. Eq. (S9) captures both the C ($\Delta_{j;lmn} = 0$) and an arbitrary IC wave ($\mathbf{q}_{j;lmn} \neq 0$ and $\Delta_{j;lmn} \neq 0$) modulated in amplitude and phase. Although $\{\Delta_{j;0},\, \Delta_{j;lmn}\} \in \mathbb{C}$ in general, we make the simplifying assumptions $\Delta_{j;0} \equiv \Delta_0 \in \mathbb{R}$, $\Delta_{j;lmn} \equiv \Delta_{lmn} \in \mathbb{R}$, $\mathbf{q}_j \parallel \mathbf{q}_j^I$, and $|\mathbf{q}_j| \equiv \eta\, q^I$, which are all compatible with the experimental density modulation $\delta\rho(\mathbf{r})$. Under these conditions, the free energy functional becomes a function of real parameters [a total of $(N+1)^3 - N^3 + 2$],

$$\mathcal{F}_{\text{cdw}}[\eta, \Delta_0, \Delta_{lmn}] \equiv \int \big[f_0(\mathbf{r}) + f_1(\mathbf{r})\big]\, d\mathbf{r}, \tag{S10}$$

where $\Delta_0$, $\Delta_{lmn}$, $\eta$, are determined to minimize $\mathcal{F}_{\text{cdw}}$ (the explicit form of $\mathcal{F}_{\text{cdw}}$ is given below).

We performed the multidimensional minimization of $\mathcal{F}_{\text{cdw}}$ numerically with respect to $\Delta_0$ and $\Delta_{lmn}$ at fixed $\eta$, subsequently scanning the latter in a fixed range. As Eq. (2) penalize deviations of $\mathbf{q}_j$ from $\mathbf{q}_j^I$ (via the $B$ term) *and* from 0 (via the $E$ term), it is sufficient to scan the range $\eta \in [0, 1]$ to obtain the global minimum. We verified that the expansion (S9) converges rapidly (cf. Fig. S2), and used the quite sufficient cutoff $N = 3$ in all subsequent calculations.

## S7.B. Explicit form of the harmonic-expanded free energy

Substituting the order parameter given by Eq. (S9) into Eq. (2) and after some algebra, the free energy can be shown to be equal to:

$$\begin{aligned}
\mathcal{F}_{\mathrm{cdw}}/3 = & \sum_{\substack{l,m,n\geq 0\\ l\cdot m\cdot n=0}} \sum_i \left[A + B(\mathbf{q}_{i;lmn} - \mathbf{q}_i^I)\cdot(\mathbf{q}_{i;l'm'n'} - \mathbf{q}_i^I) + 2\left(G + \frac{K}{2}\right)|\Delta_0|^2\right] \\
& \times \Delta_{i;lmn}\Delta^*_{i;l'm'n'}\delta(l-l', m-m', n-n') \\
& - \frac{E}{2}\sum_i \left[\Delta_{i;lmn}\Delta_{i;l'm'n'}\delta(l+l'+1, m+m', n+n') + c.c.\right] \\
& - \frac{3D}{2}\left[\Delta_{1;lmn}\Delta_{2;l'm'n'}\Delta_{3;l''m''n''}\delta(l+n'+m'', m+l'+n'', n+m'+l'') + c.c.\right] \\
& - \frac{M}{2}\sum_i \left[\Delta_{i;lmn}\Delta^*_{i+1;l'm'n'}\Delta^*_{i+2;l''m''n''}\delta(l-n'-m''+1, m-l'-n'', n-m'-l'') + c.c.\right] \\
& + G\sum_i \Delta_{i;lmn}\Delta^*_{i;l'm'n'}\Delta_{i;l''m''n''}\Delta^*_{i;l'''m'''n'''}\delta(l-l'+l''-l''', m-m'+m''-m''', n-n'+n''-n''') \\
& + \frac{K}{2}\sum_{i\neq j}\Delta_{i;lmn}\Delta^*_{i;l'm'n'}\Delta_{j;l''m''n''}\Delta^*_{j;l'''m'''n'''}\delta(l-l'+m''-m''', m-m'+n''-n''', n-n'+l''-l''') \\
& + \sum_i \left(A + B\left(q_i^I\right)^2 - E\right)|\Delta_{i;0}|^2 + \left(G + \frac{K}{2}\right)|\Delta_{i;0}|^4.
\end{aligned} \tag{S11}$$

Here, the $\delta$-function is defined as

$$\delta(l,m,n) = \begin{cases} 1, & l = m = n, \\ 0, & \text{otherwise.} \end{cases} \tag{S12}$$

In principle, complex $\Delta_{j;lmn}$'s should be used, however, as mentioned in the main text, we studied the case when $\Delta_{j;0} = \Delta_0$, $\Delta_{j;lmn} = \Delta_{lmn}$ and are real. Under these assumptions, the free energy expansion simplifies to:

$$\begin{aligned}
\mathcal{F}_{\mathrm{cdw}}/3 = & + \left(A + \tilde{B} - E\right)\Delta_0^2 + \left(G + \frac{K}{2}\Delta_0^4\right) + \sum_{\substack{l,m,n\geq 0\\ l\cdot m\cdot n=0}} \left[A + \tilde{B}\tilde{\mathbf{q}}^2_{lmn} + 2\left(G + \frac{K}{2}\right)|\Delta_0|^2\right]\Delta_{lmn}\Delta_{lmn} \\
& - E\Delta_{lmn}\Delta_{l'm'n'}\delta(l+l'+1, m+m', n+n') \\
& - D\Delta_{lmn}\Delta_{l'm'n'}\Delta_{l''m''n''}\delta(l+n'+m'', m+l'+n'', n+m'+l'') \\
& - M\Delta_{lmn}\Delta_{l'm'n'}\Delta_{l''m''n''}\delta(l-n'-m''+1, m-l'-n'', n-m'-l'') \\
& + G\Delta_{lmn}\Delta_{l'm'n'}\Delta_{l''m''n''}\Delta_{l'''m'''n'''}\delta(l-l'+l''-l''', m-m'+m''-m''', n-n'+n''-n''') \\
& + K\Delta_{lmn}\Delta_{l'm'n'}\Delta_{l''m''n''}\Delta_{l'''m'''n'''}\delta(l-l'+m''-m''', m-m'+n''-n''', n-n'+l''-l''')
\end{aligned} \tag{S13}$$

where $\tilde{\mathbf{q}}^2_{lmn} = 4\eta^2[(l^2+m^2+n^2) - (lm+ln+mn)] + 2(2l-m-n)\eta(\eta-1) + (\eta-1)^2$, with $\eta = |\boldsymbol{q}_j|/q^I$, notice that the $(q^I)^2$ has been absorbed into $\tilde{B} = B(q^I)^2$.

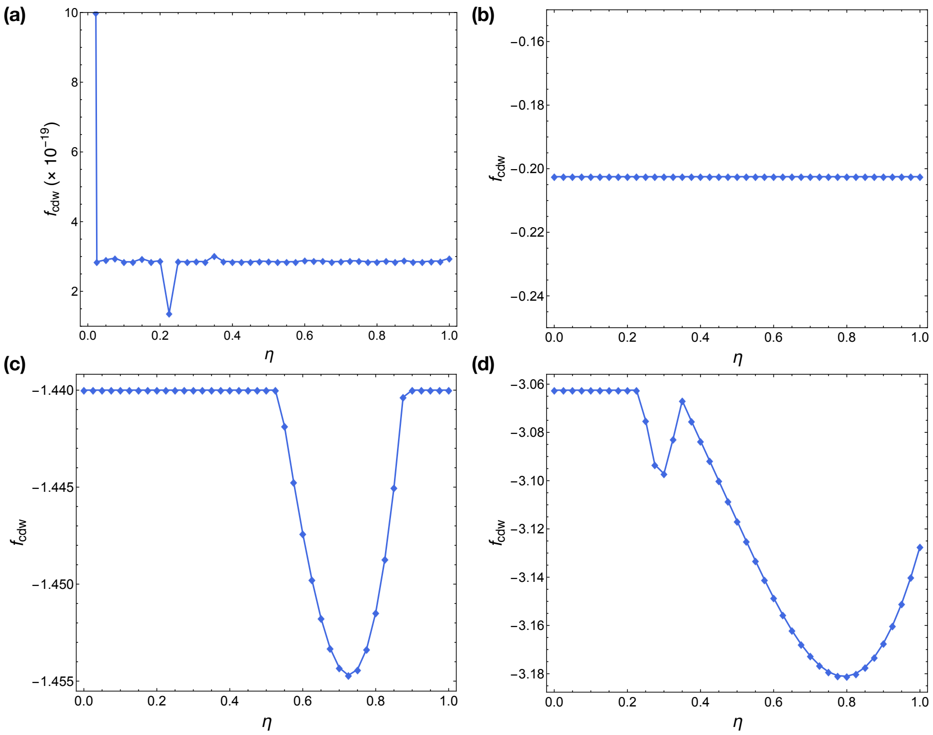


FIG. S1. Minimum of the CDW free energy (in arbitrary units) with respect to $\eta$ at $E = 2.2$. (a) For $t = 1.2$, the minimum free energy is numerically zero for all $\eta$ (note the extremely magnified vertical scale to emphasize the threshold of numerical accuracy), indicating a normal state. (b) At $t = 0.3$, the minimum of free energy is independent of $\eta$ and negative. Only the harmonic amplitude $\Delta_0$ is finite (not shown), which defines a C-CDW state. (c-d) For $t = -1.2$ and $t = -2.3$, the minimum free energy is obtained at a finite $\eta$, which implies an I-CDW state.

## S8. SOLVING FOR THE EQUILIBRIUM CDW ORDER PARAMETER

Once all the parameters of the CDW free energy are set, to find the absolute minimum of the free energy defined above, we begin by fixing $\eta$ and obtaining the saddle points in the multidimensional space spanned by the real parameters $\Delta_0$ and $\Delta_{lmn}$. The saddle points are determined by numerically solving the Euler-Lagrangian equations for $\Delta$'s. The result of this step is a curve of the minimum free energy as a function of $\eta$, $\mathcal{F}^{\min}_{\text{cdw}}(\eta)$, examples of which are shown in Fig. S1 for different effective temperatures.

The calculations require setting an harmonic cutoff $N$ that restricts the expansion to terms with $0 \leq l, m, n \leq N$. The number of variational parameters is then given by $(N+1)^3 - N^3 + 2$, which takes into account the constraint that at least one of $l, m, n$ must be zero $(l \cdot m \cdot n = 0)$, and includes $\Delta_0$ and $\eta$. The convergence of the harmonic expansion is relatively fast and we verified

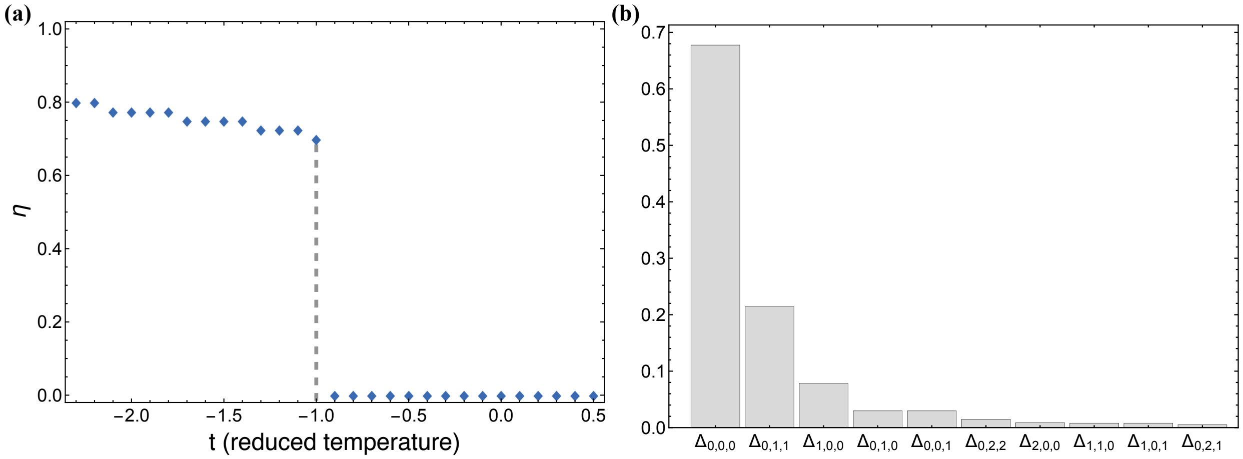


FIG. S2. Results from numerical minimization of free energy. (a) Plot of $\eta$ versus $t$ at a $E = 2.2$. The jump at $t \approx -1$ indicates a first order nature of the C-IC phase transition. (b) The ten largest $\Delta$'s at $(E, t) = (2.2, -1.7)$. Since $\Delta_{0,0,0}$ is the largest, the CDW phase is not commensurate at this point in the phase diagram.

that $N = 3$ yields a good compromise without affecting the accuracy of the results in the range of parameters studied. A typical example of the rapid decay of the higher harmonics is shown in Fig. S2(b).

Since we are minimizing numerically a 39-dimensional function, in order to reduce the chance of finding just a local minimum, we stochastically repeat each minimization multiple times (typically 200 repetitions) feeding random initial values to the minimization routine and extract the absolute minimum. Moreover, we verified that the same results are obtained with independent implementations of the minimization procedure in Mathematica and Matlab which use different algorithms for absolute minimization.

The equilibrium state is identified by the harmonic content of the order parameter for the value of $\eta$ that yields the absolute minimum of the free energy, as illustrated in Fig. S1. There are three possible outcomes: (i) If $\mathcal{F}_{\text{cdw}}^{\text{min}}(\eta) = 0$ as in Fig. S1(a), the equilibrium corresponds to the normal state, without either CCDW or ICDW. (ii) If $\mathcal{F}_{\text{cdw}}^{\text{min}}(\eta) \leq 0$ but constant with $\eta$ as in Fig. S1(b), we have a CCDW state [which is always confirmed by inspecting that $\Delta_0$ is the only non-zero component of $\psi(\mathbf{r})$]. (iii) Otherwise, $\mathcal{F}_{\text{cdw}}^{\text{min}}(\eta)$ will have a global minimum at a given $\eta$, as in the cases shown in Fig. S1(c) and Fig. S1(d), which indicates that the equilibrium state is an ICDW. As can be seen from Fig. S2(a), due to the finite jump of $\eta$ at the transition temperature, the C-IC transition is of first order.

## S9. EXPLICIT FORM OF THE SC FREE ENERGIES

As described in the main text, we considered two explicit forms of the Ginzburg-Landau free energy for the SC amplitude $\Phi(\mathbf{r})$ that differ only in whether the constant that couples it to the CDW order parameter depends on the lock-in energy $E$. In the first form the free energy in Eq. (3) reads explicitly

$$\mathcal{F}_{\rm sc} = \int \left[ \left( a_0 - a_1 \sum_j |\boldsymbol{\nabla}\psi_j|^2 \right) |\Phi|^2 + b_s |\boldsymbol{\nabla}\Phi|^2 + c_s |\Phi|^4 \right] d\mathbf{r}, \tag{S14}$$

where the constants were chosen as follows: $a_0 \equiv T = 10t + 60$, where $t$ represents the reduced temperature, $t = (T - T_{\rm icdw})/10$, here we have used the fact that $T_{\rm icdw} \approx 60$ K from the X-ray experiment[12]. In addition, the gray SC boundary in Fig. 1 was obtained by using $a_1 = 500 \times 2.1$ so that the maximum $T_{\rm sc}$ in this calculation matches the one obtained on the basis of Eq. (S15) at the calculated tip of the SC dome; $b_s = c_s = 1$ for simplicity since, presently, we are interested only in the qualitative characteristics of the solution and its relation to the DC network, and not in the specific details of how stiff the SC order parameter is, which is controlled by $b_s$, but regarding which no experimental evidence or data exists yet.

Since all constants are independent of $E$ in this scheme, the effect of the lock-in energy enters only indirectly via the dependence of the CDW texture on $E$. Using this free energy and these parameters, the SC transition occurs at the gray line shown in the phase diagram of Fig. 1.

The second scheme discussed in the main text makes the coupling depend explicitly on $E$. This means that the free energy reads explicitly

$$\mathcal{F}_{\rm sc} = \int \left[ \left( a_0 - a_1 E \sum_j |\boldsymbol{\nabla}\psi_j|^2 \right) |\Phi|^2 + b_s |\boldsymbol{\nabla}\Phi|^2 + c_s |\Phi|^4 \right] d\mathbf{r}, \tag{S15}$$

where the constants are chosen as above, $a_0 = 10t + 60$, $b_s = c_s = 1$, except that $a_1 = 500$ now. In this case, the effect of the lock-in energy $E$ appears both explicitly, as a prefactor to the interaction, and implicitly, through its effect on $\psi_j(\mathbf{r})$. It should be noted that, the value of $a_1$ here is an exaggerated one, which is chosen to show more clearly the effect of enhancement of SC order by CDW fluctuation. Actually, the position of SC dome can be tuned by changing the value of it, which will be discussed later.

## S10. ON THE COUPLING BETWEEN SUPERCONDUCTIVITY AND CDW FLUCTUATIONS

McMillan analyzed the collective modes of the discommensuration (DC) network near the commensurate-incommensurate transition in the NC regime; he considered only the phase fluctuations, approximating the amplitude as constant[2]. He had previously found that, near the transition, DCs form a spatially separated "lattice" structure[4]. The fact that this DC network is stable in the NC regime of the phase diagram implies that its low energy excitations are phonons of that emergent lattice. From the equation of motion of the small-phase fluctuations on top of the DC periodic configuration, two types of collective vibrational modes were found: a gapless mode corresponding to the collective motion of DC lattice and a gapped "phason" mode. In other words, whereas in a uniformly incommensurate state phasons are linearly dispersing gapless modes, the smaller Brillouin zone imposed by the DC superlattice in the NC regime causes the "folding" and gapping of the phase excitations that hence split into two branches.

The coupling between CDW and SC in our G-L theory is motivated precisely by this observation. Since the DCs form a periodic structure and the onset of SC correlates with the loss of commensurability across a number of transition metal dichalcogenides, it is natural to speculate that the new phonons of this emergent lattice play a role in mediating an attractive interaction between electrons ultimately leading to superconducting pairing.

Such coupling is embodied in our SC free energy of Eq. (3) in the main text. Note however that one has to generically consider both the phase, $\theta_j(\mathbf{r})$, and amplitude, $\varphi_j(\mathbf{r})$, fluctuations of the CDW order parameter[24], $\psi_j(\mathbf{r}) = \varphi_j(\mathbf{r})e^{i\theta_j(\mathbf{r})}$, and our approach takes those two into account naturally (see Figs. 2b and 2c). Therefore, our theory should couple both amplitude and phase fluctuation modes to the SC order parameter $\Phi(\mathbf{r})$. Their minimal coupling via $-a_1 \sum_j |\nabla\psi_j|^2|\Phi(\mathbf{r})|^2$ that we introduce in Eq. 2 ensures precisely that both *phason* and *amplitudon* modes couple to the SC order parameter, and the negative sign reflects the phenomenological assumption (grounded on the experimental correlation between SC and the loss of commensurability), that these fluctuations promote SC pairing [i.e., the existence of fluctuations permits lowering the total free energy with the development of a non-zero superconducting order parameter].

## S11. CHOICE OF THE SUPERCONDUCTING FREE ENERGY PARAMETERS

The key observation in relation to our modeling of the interplay between the CDW ($\psi_j$) and SC ($\Phi$) order parameters is that, experimentally, $T_{sc} \ll T_{cdw}$. Since ARPES data has established that the CDW order parameter (excitonic gap) has a mean-field-like temperature dependence[26,27], the large experimental ratio $T_{cdw}/T_{sc} \sim 20$ tells us that the onset of SC takes place at temperatures where the CDW order parameter is already at or near its $T = 0$ saturation value (see, for example, supplementary Fig. S2). In addition, as mentioned in our main text, it is experimentally known that the CDW persists in the SC phase. These two facts suggest that, in a first approximation, the emergence of SC order can be studied neglecting the self-consistent feedback that the development of this new order parameter might have in the CDW stability.

Under these conditions, the solution of the SC order parameter can proceed as if the CDW DCs texture is an independent, "externally-imposed" modulation of the superconducting pairing potential. This defines our working assumption, and means that we have now to solve a relatively conventional Ginzburg-Landau superconductivity problem, except that the quadratic coefficient in $\mathcal{F}_{\text{sc}}$, $a_s$, is an explicit function of the position. Consequently, the parameters $b_s$ and $c_s$ have the usual meaning, and determine the magnitude of the order parameter in the usual way[28]. More specifically:

1. The parameters $b_s$ and $c_s$ have no effect in the position of the SC phase boundary in the phase diagram. This is because the SC transition described by $\mathcal{F}_{\text{sc}}$ is of second order and, consequently, the transition temperature is determined entirely by the change in sign of the quadratic coefficient, $a_s$.

2. As a result of the non-uniformity of $a_s$ [via its dependence on $\boldsymbol{\nabla}\psi_j(\mathbf{r})$], regions of space where $a_s < 0$ will be superconducting, while those with $a_s > 0$ are normal. This leads to the sequence of transitions described in the section "Ramifications" of the main text, from nucleation of 0-dimensional SC dots, to proliferation (percolation) into a 1-dimensional SC network, to overall 2D superconductivity with $\Phi(\mathbf{r})$ finite everywhere.

3. The only parameter in the SC free energy with a spatial dependence is $a_s$. Therefore, the actual value of $c_s$ only determines the magnitude of $\Phi(\mathbf{r})$: the larger $c_s$ is, the smaller the overall magnitude of $\Phi(\mathbf{r})$. Hence, the magnitude of $c_s$ simply sets the scale of variation of $\Phi(\mathbf{r})$. (In practice, except when we need quantitative values of the free energy, one can always set $c_s = 1$, which corresponds to absorbing its actual magnitude by redefining the

scale of the free energy itself.)

4. The constant $b_s$ determines the stiffness of $\Phi(\mathbf{r})$. The larger it is, the more that contribution in the free energy penalizes fast spatial variations of the SC order parameter (in a type II superconductor with homogeneous pairing potential, $b_s$ controls the coherence length). If $b_s = 0$, the spatial profile of $\Phi(\mathbf{r})$ can follow precisely that of the DC network, where the localization length of $\Phi(\mathbf{r})$ coincides with the size of the DCs. In contrast, with a finite $b_s$, the localization length of $\Phi(\mathbf{r})$ will no longer be determined only by the size of the DC, but also by the magnitude of $b_s$ itself which determines how tightly $\Phi(\mathbf{r})$ can be confined within a DC. In general, an increase in $b_s$ translates into a decrease of $T_{\mathrm{sc}}$ in the NC regime due to the inhomogeneous nature of the superconducting phase in our model in this region of the phase diagram. Note, however, that although $b_s$ controls how closely the spatial extent of $\Phi(\mathbf{r})$ follows that of a DC, it does not change the fact that DCs are essential for the nucleation of the superconducting order.

For the purpose of clarity and visibility of the different phases, the phase diagram shown in the main text has been obtained with $a_0 = 10t + 60$, $t = (T - T_{\mathrm{icdw}})/10$, $a_1 = 500$. The ratio $T_{\mathrm{cdw}}/T_{\mathrm{sc}}$ in that figure underestimates the actual experimental value ($T_{\mathrm{cdw}}/T_{\mathrm{sc}} = 20$). However, the experimental ratio can easily be matched by adjusting the coupling between SC and CDW fluctuations, $a_1$. This is demonstrated explicitly in supplementary Fig. S3, where we show the effect of changing the magnitude of $a_1$ in the boundary of the SC dome. It is clear that the position of the $T_{\mathrm{sc}}$ line can be adjusted by reducing $a_1$.

## S12. SOLVING FOR THE EQUILIBRIUM SUPERCONDUCTING ORDER PARAMETER

We must determine the solution $\Phi(\mathbf{r})$ that minimizes the free energy $\mathcal{F}_{\mathrm{sc}}$ in either of the forms written in (S14) or (S15). For every point $(E, t)$ in the parameter space of the phase diagram, we replace $\psi_j(\mathbf{r})$ by the corresponding equilibrium solution arising from the minimization of $\mathcal{F}_{\mathrm{cdw}}$. Since $\psi_j(\mathbf{r})$ is non-uniform in space outside the C-CDW phase, this turns the equations (S14) and (S15) into non-uniform Ginzburg-Landau problems.

Numerically, we solve the Euler-Lagrange equations for $\Phi(\mathbf{r})$ using the CDW texture ($\sum_j |\nabla\psi_j(r)|^2$) itself as the initial trial solution which is then relaxed under periodic boundary conditions consistent with the CDW and DC network.

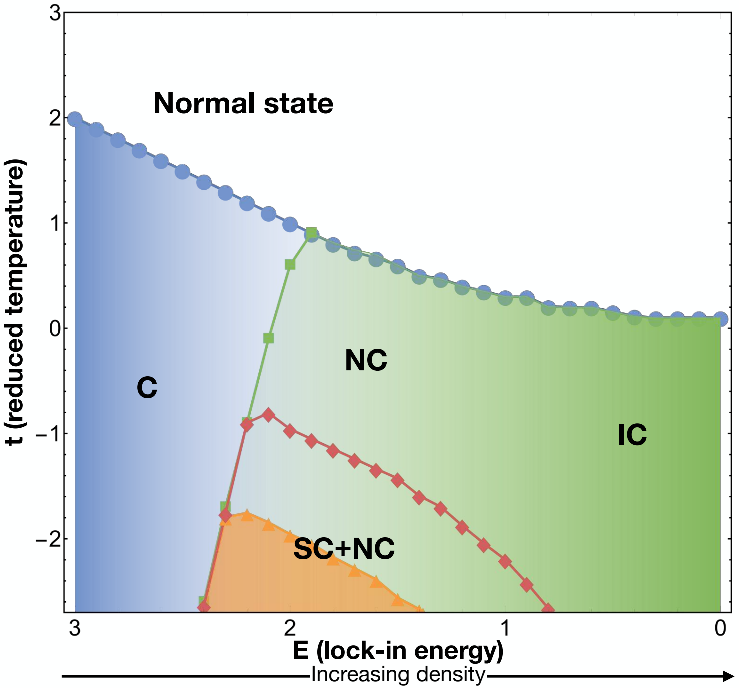


FIG. S3. Phase diagram of the G-L model emphasizing how the parameter $a_1$ in the superconducting free energy $\mathcal{F}_{\rm sc}$ determines the position of the SC phase boundary within the NC region. The red line is the same shown in Fig. 1 of the main text, and has been obtained with $a_1 = 500$. The orange line marks the same SC boundary, but obtained with a smaller value, $a_1 = 250$.

## S13. REAL-SPACE SUPERCONDUCTING ORDER

Fig. S4 shows the real space SC order in different cases that correspond to the solutions that minimize the total free energy in different regions of the $(E, t)$ parameter space. temperature right below the $T_{\rm sc}^{(0)}$, isolated SC islands emerge at the intersection of three CDW DCs and forms a Kagome lattice, as shown in panel (a1-2). At very low temperature ($T < T_{\rm sc}^{(2)}$), the area of SC network expands and is able to cover the entire space, a 2D SC regime is achieved. Due to the linear dependence on $E$ in the CDW and SC coupling $a_1$, when $E$ decreases, the SC order gets suppressed so one can get the dome shape of SC phase as shown in the phase diagram from main text. If the $E$-dependence is removed, in the IC phase (with very small $E$), because of the strong fluctuation of CDW order parameter (relative to CCDW), it can still support a SC order, as shown in panel Fig. S4(d1-2).

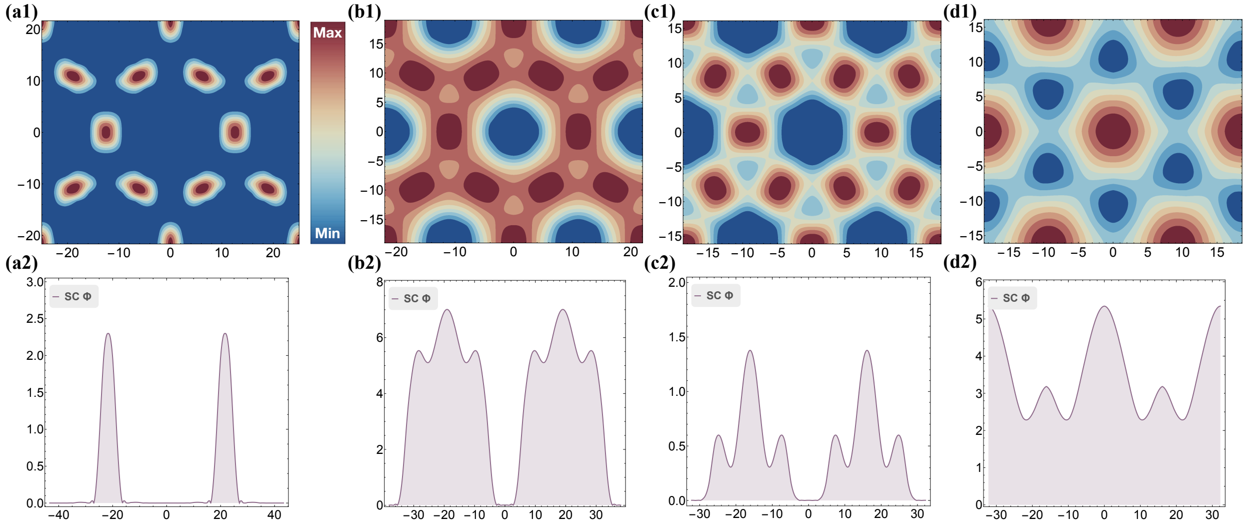


FIG. S4. Real space plots of the SC order parameter, $\Phi(\mathbf{r})$, computed for the CDW state at specific points $(E,t)$ of the phase diagram shown in Fig. 1 of the main text. Each panel in the bottom row shows a vertical section along the line $x=0$ of the density plot directly above it. (a) $(E,t)=(2.2,-1.1)$: right below $T_{\rm sc}^{\rm 0d}$, SC order nucleates on isolated 0d regions that coincide with the vertices of the Kagome lattice defined by the intersection of DCs. (b) $(E,t)=(2.2,-3)$: reducing the temperature from $T_{\rm sc}^{\rm 0d}$, stabilizes the SC state further. Both the amplitude and spatial extent of the SC order parameter increase monotonically. The case shown corresponds to a temperature below the percolation threshold, $T<T_{\rm sc}^{\rm 1d}$. (c) $(E,t)=(1,-2.4)$: the linear dependence of the CDW-SC coupling constant $a_s$ with $E$ weakens the SC amplitude when the lock-in energy is reduced. (d) $(E,t)=(0,-2)$: unlike the previous cases, here $\Phi(\mathbf{r})$ has been obtained using an $E$-independent coupling $a_s$, as described in the text in relation to the gray SC boundary line in Fig. 1. With no lock-in energy ($E=0$), the equilibrium CDW solution approximates a homogeneously IC state (i.e., one without DCs). SC is therefore stabilized over the whole system.

[1] K. Nakanishi and H. Shiba, J. Phys. Soc. Jpn. **43**, 1839 (1977).

[2] W. L. McMillan, Phys. Rev. B **16**, 4655 (1977).

[3] A. E. Jacobs and M. B. Walker, Phys. Rev. B **21**, 4132 (1980).

[4] W. L. McMillan, Phys. Rev. B **14**, 1496 (1976).

[5] D. E. Moncton, J. D. Axe, and F. J. Disalvo, Phys. Rev. Lett. **34**, 734 (1975).

[6] B. Sipos, A. F. Kusmartseva, A. Akrap, H. Berger, L. Forró, and E. Tutiš, Nat. Mater. **7**, 960 (2008).

[7] M. Leroux, I. Errea, M. Le Tacon, S.-M. Souliou, G. Garbarino, L. Cario, A. Bosak, F. Mauri, M. Calandra, and P. Rodière, Phys. Rev. B **92**, 140303 (2015).

[8] D. B. McWhan, R. M. Fleming, D. E. Moncton, and F. J. DiSalvo, Phys. Rev. Lett. **45**, 269 (1980).

[9] A. H. Castro Neto, Phys. Rev. Lett. **86**, 4382 (2001).

[10] W. L. McMillan, Phys. Rev. B **12**, 1187 (1975).

[11] Y. I. Joe, X. M. Chen, P. Ghaemi, K. D. Finkelstein, G. a. de la Peña, Y. Gan, J. C. T. Lee, S. Yuan, J. Geck, G. J. MacDougall, T. C. Chiang, S. L. Cooper, E. Fradkin, and P. Abbamonte, Nat. Phys. **10**, 421 (2014), 1309.4051.

[12] A. Kogar, G. A. de la Pena, S. Lee, Y. Fang, S. X.-L. Sun, D. B. Lioi, G. Karapetrov, K. D. Finkelstein, J. P. C. Ruff, P. Abbamonte, and S. Rosenkranz, Phys. Rev. Lett. **118**, 027002 (2017).

[13] L. J. Li, E. C. T. O'Farrell, K. P. Loh, G. Eda, B. Özyilmaz, and A. H. Castro Neto, Nature **529**, 185 EP (2015).

[14] A. M. Novello, M. Spera, A. Scarfato, A. Ubaldini, E. Giannini, D. R. Bowler, and C. Renner, Phys. Rev. Lett. **118**, 017002 (2017).

[15] S. Yan, D. Iaia, E. Morosan, E. Fradkin, P. Abbamonte, and V. Madhavan, Phys. Rev. Lett. **118**, 106405 (2017).

[16] K. Nakanishi and H. Shiba, J. Phys. Soc. Jpn. **44**, 1465 (1978).

[17] P. A. Lee, T. M. Rice, and P. W. Anderson, Solid State Commun. **14**, 703 (1974).

[18] A. Kotani, J. Phys. Soc. Jpn. **42**, 408 (1977).

[19] A. Kotani, J. Phys. Soc. Jpn. **42**, 416 (1977).

[20] See Supplemental Material at [URL will be inserted by publisher], which includes references[1–28].

[21] C. Chen, B. Singh, H. Lin, and V. M. Pereira, Phys. Rev. Lett. **121**, 226602 (2018).

[22] K. Nakanishi and H. Shiba, J. Phys. Soc. Japan **45**, 1147 (1978).

[23] P. Bak and V. J. Emery, Phys. Rev. Lett. **36**, 978 (1976).

[24] S. A. Jackson, P. A. Lee, and T. M. Rice, Phys. Rev. B **17**, 3611 (1978).

[25] K. Nakanishi, H. Takater, Y. Yamada, and H. Shiba, J. Phys. Soc. Jpn. **43**, 1509 (1977).

[26] C. Monney, E. F. Schwier, M. G. Garnier, N. Mariotti, C. Didiot, H. Cercellier, J. Marcus, H. Berger, A. N. Titov, H. Beck, and P. Aebi, New J. Phys. **12**, 125019 (2010).

[27] P. Chen, Y.-H. Chan, X.-Y. Fang, Y. Zhang, M.-Y. Chou, S.-K. Mo, Z. Hussain, A.-V. Fedorov, and T.-C. Chiang, Nat. Commun. **6**, 8943 (2015).

[28] M. Tinkham, *Introduction to Superconductivity: Second Edition* (McGraw Hill, Inc., New York, 1996).
